# Supplementary material for: Nonparametric Bootstrap Inference for the Targeted Highly Adaptive LASSO Estimator
Source: arXiv:1905.10299 source file (2020-02-07)
Supplement: Supplementary file 1 [file appendix_mark.tex]

Check that results are not only for $d_{01}$ but also for ${\bf d}_{01}$ but now in terms of vector ${\bf L}_1$. Same for $d_{02}$. 
State that also in lemma. 

\section{Proof that $Q_n^*$ preservation  rate of convergence of $Q_n$}
The following lemma establishes that $Q_n^*$ preserves the rate of convergence of $Q_n$. 
%We now want show that $d_{01}(Q_n^*,Q_0)$ is close to $d_{01}(Q_n,Q_0)$.
\begin{lemma}\label{lemmathalmle}
Assume $\epsilon\rightarrow L_1(Q_{n,\epsilon})$ is differentiable with a uniformly bounded derivative on an interval $\epsilon \in (-\delta,\delta)$ for some $\delta>0$.
Define $\epsilon_{0n}=\arg\min_{\epsilon}P_0 L_1(Q_{n,\epsilon})$ and assume the weak regularity condition  
\begin{equation}\label{Qnstarconv}
\epsilon_{0n}=O_P(d_{01}^{0.5}(Q_n,Q_0)).\end{equation}
Then,
\begin{equation}\label{thalmle}
d_{01}(Q_n^*,Q_0)\leq d_{01}(Q_n,Q_0)+O_P(n^{-1/2-\alpha(d)}).\end{equation}
Specifically,
\begin{eqnarray*}
d_{01}(Q_n^*,Q_0)&\leq& -(P_n-P_0)L_1(Q_{n,\epsilon_{0n}},Q_n)-(P_n-P_0)L_1(Q_n,Q_0)\\
&=&-(P_n-P_0)\{L_1(Q_{n,\epsilon_{0n}},Q_n)+L_1(Q_n,Q_0)\}\\
&=&-(P_n-P_0)L_1(Q_{n,\epsilon_{0n}},Q_0) .
\end{eqnarray*}
Under a weak regularity condition, we have $\epsilon_n-\epsilon_{0n}=O_P(n^{-1/2})$.
Then,
\[
d_{01}(Q_n^*,Q_0)\leq -(P_n-P_0)L_1(Q_n^*,Q_0)+O_P(n^{-1}).\]
\end{lemma}
This also proves that the iterative TMLE using a {\em finite} (uniform in $n$) number of iterations satisfies $d_{01}(Q_n^*,Q_0)\leq d_{01}(Q_n,Q_0)+O_P(n^{-1/2-\alpha(d)})$. So  if needed  one can iterate the TMLE to guarantee that $r_n$ is small enough to be neglected. 
\newline
{\bf Proof:}
%Define $\epsilon_{0n}=\arg\min_{\epsilon}P_0 L_1(Q_{n,\epsilon})$.
Using the MLE properties of $\epsilon_{0n}$ and $Q_n$, we obtain
\begin{eqnarray*}
P_0L_1(Q_n^*)-P_0L_1(Q_0)&=&\{ P_0L_1(Q_{n,\epsilon_n}-P_0L_1(Q_{n,\epsilon_{0n}})\}
+\{P_0L_1(Q_{n,\epsilon_{0n}})-P_0L_1(Q_n)\}\\
&&+\{P_0L_1(Q_n)-P_0L_1(Q_0)\}\\
&\leq & P_0L_1(Q_{n,\epsilon_{0n}},Q_n) +\{P_0L_1(Q_n)-P_0L_1(Q_0)\}\\
&=&(P_0-P_n)L_1(Q_{n,\epsilon_{0n}},Q_n) +P_n L_1(Q_{n,\epsilon_{0n}},Q_n)+d_{01}(Q_n,Q_0)\\
&\leq &-(P_n-P_0)L_1(Q_{n,\epsilon_{0n}},Q_n)+d_{01}(Q_n,Q_0)\\
&=&-(P_n-P_0)L_1(Q_{n,\epsilon_{0n}},Q_0).
\end{eqnarray*}

An exact first order Tailor expansion $f(\epsilon_{0n})-f(0)=\frac{d}{d\xi}f(\xi)\epsilon_{0n}$ for a $\xi$ between $0$ and $\epsilon_{0n}$, we obtain
\[
L_1(Q_{n,\epsilon_{0n} })-L_1(Q_{n})=\epsilon_{0n}\frac{d}{d\xi }L_1(Q_{n,\xi} ).\]
Using that $\epsilon_{0n}$ converges as fast to zero as $d_{01}(Q_n,Q_0)$ and that it is an empirical process indexed by  the Donsker class of cadlag functions with sectional variation norm bounded by universal $M_1$, 
it then follows that $(P_n-P_0)L_1(Q_{n,\epsilon_{0n}},Q_n)=O_P(n^{-1/2-\alpha(d)})$, analogue to analysis of HAL-MLE. So we have
\[
d_{01}(Q_n^*,Q_0)\leq d_{01}(Q_n,Q_0)+O_P(n^{-1/2-\alpha(d)}) .\]
It remains to prove the last claim. We have \[
(P_n-P_0)L_1(Q_{n,\epsilon_{0n}},Q_0)=(P_n-P_0)L_1(Q_{n,\epsilon_{0n}},Q_{n,\epsilon_n})+(P_n-P_0)L_1(Q_n^*,Q_0).\]
We can do an exact tailor expansion at $\epsilon_{0n}$ of the first term so that we obtain $(\epsilon_n-\epsilon_{0n})(P_n-P_0)\frac{d}{d\xi}L_1(Q_{n,\xi})$ at $\xi$ between $\epsilon_n$ and $\epsilon_{0n}$. The latter term is $O_P(n^{-1})$.
$\Box$ 

\section{Proof of Theorem \ref{thnpbootmle}.}

To prove this theorem, we first present the following straightforward lemma, which follows immediately by just imitating the proof of the convergence of the HAL-MLE $Q_n$ itself.

\begin{lemma}\label{generalhalmle}
We have
\begin{eqnarray}
0&\leq & d_{n1}(Q_n^{\#},Q_n)\equiv P_n\{ L_1(Q_n^{\#})-L_1(Q_n)\}\nonumber \\
&=& -(P_n^{\#}-P_n)\{L_1(Q_n^{\#})-L_1(Q_n)\}+P_n^{\#}\{L_1(Q_n^{\#})-L_1(Q_n)\}\nonumber \\
&\leq& -(P_n^{\#}-P_n)\{L_1(Q_n^{\#})-L_1(Q_n)\},\label{boota}
\end{eqnarray}
and similarly $d_{n2}(G_n^{\#},G_n)\leq -(P_n^{\#}-P_n)L_2(G_n^{\#},G_n)$.
As a consequence, we have $d_{n1}(Q_n^{\#},Q_n)=P_n L_1(Q_n^{\#})-P_nL_1(Q_n)$
 and $d_{n2}(G_n^{\#},G_n)=P_n L_2(G_n^{\#})-P_nL_2(G_n)$ are both $O_P(n^{-1/2})$.
In addition, since $L_1(Q_n^{\#})-L_1(Q_n)$ falls in a uniform Donsker class with probability 1 so that the empirical process is asymptotically equicontinuous, we have that if  $d_{n1}(Q_n^{\#},Q_n)\rightarrow 0$ and $d_{n2}(G_n^{\#},G_n)\rightarrow 0$ implies that $P_n \{L_1(Q_n^{\#})-L_1(Q_n)\}^2\rightarrow 0$ and $P_n \{L_2(G_n^{\#})-L_2(G_n)\}^2\rightarrow 0$, 
then we have $d_{n1}(Q_n^{\#},Q_n)=o_P(n^{-1/2})$ and $d_{n2}(G_n^{\#},G_n)=o_P(n^{-1/2})$.
If these dissimilarities are equivalent in the sense that  $\pl L_1(Q_n^{\#})-L_1(Q_n)\pl_{P_n}^2\lesssim d_{n1}(Q_n^{\#},Q_n)$, then we have 
$d_{n1}(Q_n^{\#},Q_n)=O_P(n^{-1/2-\alpha(d)})$ and similarly for $G_n^{\#}$.
\end{lemma}

%The above lemma is completely general and demonstrates the HAL-MLE  on a bootstrap sample is still consistent at a same rate as the original HAL-MLE on the original data, but it is now w.r.t. the loss-based dissimilarity $d_{n1}(Q_n^{\#},Q_n)$. The question is if this type of $d_{n1}$ and $d_{n2}$-consistency of $Q_n^{\#}$  and $G_n^{\#}$ w.r.t. $Q_n$ and $G_n. In order to derive some concrete results we focus now on the case that the parameter spaces for $Q$ and $G$ are nonparametric sets of cadlag functions with a uniformly bounded sectional variation norm.  So $Q_n=\arg\min_{Q\in D[0,\tau_1],\pl Q\pl_v^*<M_1}P_n L_1(Q)$ and $Q_n^{\#}=\arg\min_{Q\in D[0,\tau_1],\pl Q\pl_v^*<M_1}P_n^{\#}L_1(Q)$ and similarly $G_n=\arg\min_{G\in D[0,\tau_2],\pl G\pl_v^*<M_2}P_n L_2(G)$ and $G_n^{\#}=\arg\min_{G\in D[0,\tau_1],\pl G\pl_v^*<M_2}P_n^{\#}L_2(G)$.

The following lemma establishes that $d_{n1}(Q_n^{\#},Q_n)$ is equivalent with a square of an $L^2(P_n)$-norm of a difference of  $Q_n^{\#}$ and $Q_n$.
Of course, this lemma is equally applicable to $d_{n2}(G_n^{\#},G_n)$. We start with presenting the specific result for the case that $L_1(Q)$ is the squared error loss, even though this result is a consequence of our general result.

\begin{lemma}\label{bootstrapHALMLEstructure}
Suppose that $L_1(Q)(O)=(Y-Q(X))^2$ is the squared error loss. Then,
we have
\[
0\leq d_{n1}(Q_n^{\#},Q_n)\geq P_n (Q_n^{\#}-Q_n)^2 .\]
Since  $P_n  \{L_1(Q_n^{\#})-L_1(Q_n)\}^2\lesssim P_n (Q_n^{\#}-Q_n)^2$, this implies
$P_n  \{L_1(Q_n^{\#})-L_1(Q_n)\}^2\lesssim d_{n1}(Q_n^{\#},Q_n)$.
Combined with (\ref{boota}) and empirical process theory, this shows 
\[
d_{n1}(Q_n^{\#},Q_n)=O_P(n^{-1/2-\alpha(d)}).
\]
This, on its turn then implies  $P_n (Q_n^{\#}-Q_n)^2=O_P(n^{-1/2-\alpha(d)})$.

For general loss, consider the following assumptions. Suppose that $L_1(Q)$ is differentiable at $Q=Q_n$ so that
\[
P_n \{L_1(Q_n^{\#})-L_1(Q_n)\}=P_n \frac{d}{dQ_n}L_1(Q_n)(Q_n^{\#}-Q_n)+P_n R_{2L_1,n}(Q_n^{\#},Q_n)\]
for some second order term $R_{2L_1,n}(Q_n^{\#},Q_n)$ involving square differences between $Q_n^{\#}$ and $Q_n$. We have $P_n\frac{d}{dQ_n}L_1(Q_n)(Q_n^{\#}-Q_n)\geq 0$ so that  
\[
0\leq d_{n1}(Q_n^{\#},Q_n) \geq P_n R_{2L_1,n}(Q_n^{\#},Q_n).\]
We will typically have \[
P_n \{L_1(Q_n^{\#})-L_1(Q_n)\}^2\lesssim P_nR_{2L_1,n}(Q_n^{\#},Q_n),\]
which we assume to hold, which  then implies 
\[
P_n \{L_1(Q_n^{\#})-L_1(Q_n)\}^2\lesssim d_{n1}(Q_n^{\#},Q_n).\]
Combined with (\ref{boota}) and empirical process theory, this shows
\[
0\leq d_{n1}(Q_n^{\#},Q_n)=O_P(n^{-1/2-\alpha(d)}).\]
This, on its turn then  implies
 $P_nR_{2L_1,n}(Q_n^{\#},Q_n)=O_P(n^{-1/2-\alpha(d)})$.
\end{lemma}
{\bf Proof:}
We first prove the results for the general loss function, and subsequently, we will consider the special case that $L_1(Q)$ is the squared error loss.
Consider the  path  $Q_{n,\epsilon}(x)=(1+\epsilon h(0))Q_n(0)+\sum_s \int_{(0_s,x_s]}(1+\epsilon h_s(u_s)) dQ_{n,s}(u_s))$ for $\epsilon \in [0,\delta)$ for some $\delta>0$, where $r(h,Q_n)\equiv  h(0)\mid Q_n(0)\mid+\sum_s \int_{(0_s,\tau_s]} h_s(u_s)\mid dQ_{n,s}(u_s)\mid \leq 0$ and $h$ is uniformly bounded.  Let ${\cal H}$ be the set of $h$ functions (i.e., functions of $s,u_s$).
For $\epsilon$ small enough we have $(1+\epsilon h(0))>0$ and $1+\epsilon h_s(u_s)>0$. Thus, for $\epsilon$ small enough we have
\begin{eqnarray*}
\pl Q_{n,\epsilon}\pl_v^*&=&(1+\epsilon h(0))\mid Q_n(0)\mid+\sum_s \int_{(0_s,\tau_s]}(1+\epsilon h_s(u_s))\mid dQ_{n,s}(u_s)\mid \\
&=& \pl Q_n\pl_v^*+\epsilon\left\{ h(0)\mid Q_n(0)\mid+\sum_s \int_{(0_s,\tau_s]}h_s(u_s) \mid dQ_{n,s}(u_s)\mid \right\} \\
&=&\pl Q_n\pl_v^*+\epsilon r(h,Q_n)\\
&\geq & \pl Q_n\pl_v^*,
\end{eqnarray*}
by assumption that $r(h,Q_n)\leq 0$ and $\epsilon>0$.
Thus, for a small enough $\delta>0$ $\{Q_{n,\epsilon}:0\leq \epsilon<\delta\}$ represents a path of cadlag functions with sectional variation norm  smaller than or equal to $M=\pl Q_n\pl_v^*$. In addition, we have that $dQ_{n,s}(u_s)=0$ implies $(1+\epsilon h_s(u_s))dQ_{n,s}(u_s)=0$ so that the support of $Q_{n,\epsilon}$ is included in the support $A$ of $Q_n$. Thus, this proves that for $\delta>0$ small enough this path is indeed a  submodel of ${\cal F}_{1,A}^{np}$ with $C_1=\pl Q_n\pl_v^*$, where we note that $\pl Q_n\pl_v^*$ attains its maximal allowed value $C_1$.
We also have that
 \[
 Q_{n,\epsilon}-Q_n=\epsilon\left\{ Q_n(0)h(0)+ \sum_s \int_{(0_s,x_s]} h_s(u_s)dQ_{n,s}(u_s))\right\} .\]
 Thus,
 \[
 \frac{d}{d\epsilon}Q_{n,\epsilon}=f(h,Q_n)\equiv Q_n(0)h(0)+ \sum_s \int_{(0_s,x_s]} h_s(u_s)dQ_{n,s}(u_s)) .\]
 %Note that $f(h,Q_n)$ represents a difference of two cadlag functions.
 Let ${\cal S}\equiv \{f(h,Q_n): h\in {\cal H}\}$.
 By definition of the MLE $Q_n$, we also have that $\epsilon \rightarrow P_n L_1(Q_{n,\epsilon})$ is minimal over $[0,\delta)$ at $\epsilon =0$. 
This shows that the derivative of $P_n L_1(Q_{n,\epsilon})$ from the right at $\epsilon =0$ is  non-negative:
 \[
 \frac{d}{d\epsilon+ }P_n L_1(Q_{n,\epsilon })\geq 0\mbox{ at $\epsilon =0$}.\]
 This derivative is given by $P_n \frac{d}{dQ_n}L_1(Q_n)(f(h,Q_n))$, where $d/dQ_nL_1(Q_n)(f(h,Q_n))$ is the directional derivative in direction $f(h,Q_n)$.
  Thus for each $h\in {\cal H}$, we have
\[
P_n \frac{d}{dQ_n}L_1(Q_n)(f(h,Q_n)) \geq 0 .\]
Suppose that
\begin{equation}\label{keya1}
Q_n^{\#}-Q_n\in {\cal S}=\{f(h,Q_n):h\in {\cal H}\}.\end{equation}
Then, we have
\[
P_n \frac{d}{dQ_n}L_1(Q_n)(Q_n^{\#}-Q_n)\geq 0.\]
Combined with the assumed differentiability of $P_n L_1(Q)$ at $Q=Q_n$ with second order remainder $P_nR_{2L_1,n}(Q_n^{\#},Q_n)$, this proves
%\[P_n \{L_1(Q_n^{\#})-L_1(Q_n)\}=P_n \frac{d}{dQ_n}L_1(Q_n)(Q_n^{\#}-Q_n)+R_2(Q_n^{\#},Q_n)\]for some second order remainder involving square differences between $Q_n^{\#}$ and $Q_n$. Then,
\[
0\leq P_n\{L_1(Q_n^{\#})-L_1(Q_n)\}\geq P_nR_{2L_1,n}(Q_n^{\#},Q_n).\]
Thus it remains to show (\ref{keya1}).

% Since $\pl Q_n^\#}\pl_v^*=\pl Q_n\pl_v^*=M$ will both achieve the maximal allowed variation norm, and  $Q_{n,s}^{\#}\ll Q_{n,s}$ for all subset $s$ (i.e., the support of $Q_{n,s}^{\#}$ is a subset of the support of $Q_{n,s}$ due to the support of $P_n^{\#}$ being  a subset of support of $P_n$), one would generally expect that indeed this difference $Q_n^{\#}-Q_n$ is included in ${\cal S}$.
In order to prove (\ref{keya1}), let's solve explicitly for $h$ so that $Q_n^{\#}-Q_n=f(h,Q_n)$ and then verify that $h\in {\cal H}$ satisfies its assumed constraints (i.e., $r(h,Q_n)\leq 0$ and uniformly bounded).
We have
\begin{eqnarray*}
Q_n^{\#}-Q_n&=&Q_n^{\#}(0)-Q_n(0)+\sum_s\int_{(0_s,x_s]} d(Q_{n,s}^{\#}-dQ_{n,s})(u_s)\\
&=& Q_n^{\#}(0)-Q_n(0)+\sum_s \int_{(0_s,x_s]} \frac{d(Q_{n,s}^{\#}-dQ_{n,s})}{dQ_{n,s}} dQ_{n,s}(u_s),
\end{eqnarray*}
where we used that $Q_{n,s}^{\#}\ll Q_{n,s}$ for each subset $s$, since the support of the bootstrap sample is  a subset of  the support $\{O_1,\ldots,O_n\}$ of $P_n$.
Let $h(Q_n^{\#},Q_n)$ be defined by
\begin{eqnarray*}
h(Q_n^{\#},Q_n)(0)&=&(Q_n^{\#}(0)-Q_n(0))/Q_n(0)\\
h_s(Q_n^{\#},Q_n)&=&\frac{d(Q_{n,s}^{\#}-dQ_{n,s})}{dQ_{n,s}}\mbox{ for all subset $s$} .
\end{eqnarray*}
For this choice $h(Q_n^{\#},Q_n)$, we have $f(h,Q_n)=Q_n^{\#}-Q_n$.
We now need to verify if  $r(h,Q_n)\leq 0$ for this choice $h(Q_n^{\#},Q_n)$.
We have
\begin{eqnarray*}
r(h,Q_n)&=&\frac{Q_n^{\#}(0)-Q_n(0)}{Q_n(0)}\mid Q_n(0)\mid+\sum_s\int_{(0_s,\tau_s]}\frac{dQ_{n,s}^{\#}-dQ_{n,s}}{dQ_{n,s}}\mid dQ_{n,s}\mid\\
&=&I(Q_n(0)>0)\{Q_n^{\#}(0)-Q_n(0)\}+I(Q_n(0)\leq 0)\{Q_n(0)-Q_n^{\#}(0)\}\\
&&+\sum_s\int_{(0_s,\tau_s]}I(dQ_{n,s}\geq 0) d(Q_{n,s}^{\#}-dQ_{n,s})\\
&&+\sum_s\int_{(0_s,\tau_s]} I(dQ_{n,s}<0)d(Q_{n,s}-Q_{n,s}^{\#})\\
&=&-\pl Q_n\pl_v^*+Q_n^{\#}(0)\{ I(Q_n(0)>0)-I(Q_n(0)\leq 0)\} \\
&&+\sum_s \int_{(0_s,\tau_s]}\{I(dQ_{n,s}\geq 0) -I(dQ_{n,s}\leq 0\} dQ_{n,s}^{\#}\\
&\leq&-\pl Q_n\pl_v^*+\mid Q_n^{\#}(0)\mid +\sum_s\int_{(0_s,\tau_s]} \mid dQ_{n,s}^{\#}(u_s)\mid \\
&=&-\pl Q_n\pl_v^*+\pl Q_n^{\#}\pl_v^*\\
&\leq &0,
\end{eqnarray*}
since $\pl Q_n^{\#}\pl_v^*\leq M=\pl Q_n\pl_v^*$.
Thus, this proves that indeed $r(h,Q_n)\leq 0$ and thus that $Q_n^{\#}-Q_n\in {\cal S}$.
This proves (\ref{keya1}) and thereby the general loss-function statements of the lemma.

Consider  now the squared error loss $L_1(Q)=(Y-Q(X))^2$. Then,
\begin{eqnarray*}
d_{n1}(Q_n^{\#},Q_n)&=&\frac{1}{n}\sum_i \{2Y_iQ_n(X_i)-2Y_i Q_n^{\#}(X_i)+Q_n^{\#2}(X_i)-Q_n^2(X_i)\}\\
&=& \frac{1}{n}\sum_i\{2  (Q_n-Q_n^{\#})(X_i)  Y_i+Q_n^{\#2}(X_i)-Q_n^2(X_i)\}\\
&=&\frac{1}{n}\sum_i \{2(Q_n-Q_n^{\#})(X_i)(Y_i-Q_n(X_i))\\
&&+2(Q_n-Q_n^{\#})Q_n(X_i)+Q_n^{\#2}(X_i)-Q_n^2(X_i)\}\\
&=&\frac{1}{n}\sum_i 2(Q_n-Q_n^{\#})(X_i)(Y_i-Q_n(X_i))+\frac{1}{n}\sum_i (Q_n-Q_n^{\#})^2(X_i).\end{eqnarray*}
Note that the first term corresponds with $P_n\frac{d}{dQ_n}L_1(Q_n)(Q_n^{\#}-Q_n)$ and the second order term with $P_nR_{2L_1,n}(Q_n^{\#},Q_n)$, where
$R_{2L_1,n}(Q_n^{\#},Q_n)=(Q_n^{\#}-Q_n)^2$.
We want to show that $ \frac{1}{n}\sum_i 2(Q_n-Q_n^{\#})(X_i)(Y_i-Q_n(X_i))\geq 0$.
The general equation above $P_n \frac{d}{dQ_n}L_1(Q_n)(f(h,Q_n)) \geq 0$ corresponds for the squared error loss with:
\[
-2 \frac{1}{n}\sum_i f(h,Q_n)(Y_i-Q_n(X_i)) \geq 0.\]
As we showed in general above  we have that $f(h,Q_n)$ can be chosen to be equal to $Q_n^{\#}-Q_n$.
So this proves that $n^{-1}\sum_i(Q_n^{\#}-Q_n)(X_i)(Y_i-Q_n(X_i))\leq 0$. This proves the desired result for the squared error loss.
Specifically,
\[
d_{n1}(Q_n^{\#},Q_n)\geq P_n (Q_n-Q_n^{\#})^2.\]
Clearly, $P_n  \{L_1(Q_n^{\#})-L_1(Q_n)\}^2\leq C P_n (Q_n^{\#}-Q_n)^2\leq Cd_{n1}(Q_n^{\#},Q_n)$ for some $C<\infty$. 
As a consequence, applying empirical process results (van der Vaart, Wellner) to (\ref{boota}) yields now\[
d_{n1}(Q_n^{\#},Q_n)=O_P(n^{-1/2-\alpha(d)}).\]
This completes the proof of all statements in the lemma. $\Box$

The next lemma proves the last statement in Theorem \ref{thnpbootmle}.
\begin{lemma}\label{dndo}
%The question is then if the desired convergence in this $L^2(P_n)$-norm also implies this same rate of convergence w.r.t. $L^2(P_0)$-norm. 
Suppose that $\int f^2_n dP_n=O_P(n^{-1/2-\alpha(d)})$ and we know that $\pl f_n\pl_v^*<M$ for some $M<\infty$. 
Then $\int f_n^2dP_0=O_P(n^{-1/2-\alpha(d)})$.
\end{lemma}
{\bf Proof:}
We have 
\begin{eqnarray*}
\int f_n^2 dP_0&=&\int f_n^2d(P_n-P_0)+\int f_n^2 dP_n\\
&=&\int f_n^2 d(P_n-P_0)+O_P(n^{-1/2-\alpha(d)}).
\end{eqnarray*}
We have $\int f_n^2 d(P_n-P_0)=O_P(n^{-1/2})$.
This proves that $\int f_n^2 dP_0=O_P(n^{-1/2})$. By asymptotic equicontinuity of the empirical process indexed by cadlag functions with uniformly bounded sectional variation norm, it follows now also that $\int f_n^2 d(P_n-P_0)=O_P(n^{-1/2-\alpha(d)})$. Thus, this proves that indeed
that $\int f_n^2 dP_0=O_P(n^{-1/2-\alpha(d)})$ follows from $\int f_n^2dP_n=O_P(n^{-1/2-\alpha(d)})$.
$\Box$

\section{Preservation of rate for bootstrapped targeted estimator}
In our theorem we just assumed $\epsilon_n^{\#2}=O_P(n^{-1/2-\alpha(d)})$.
Below, we show that under regularity conditions, indeed $d_{10}(Q_{n,\epsilon_n^{\#}}^{\#},Q_0)=O_P(n^{-1/2-\alpha(d)})$.
As the following proof demonstrates, if $\epsilon\rightarrow  L_1(Q_{\epsilon})$ is twice differentiable, and the minima $\tilde{\epsilon}_n^{\#}$ of $P_n L_1(Q_{n,\epsilon}^{\#})$ and $\epsilon_{0,n}^{\#}$ of $P_0L_1(Q_{n,\epsilon}^{\#})$ are interior minima with derivative equal to zero, then
$d_{01}(Q_{n,\epsilon_n^{\#}}^{\#},Q_0)=O_P(n^{-1/2-\alpha(d)})$.

Recall that $\sup_{\epsilon}\pl Q_{\epsilon}\pl_v^*< C \pl Q\pl_v^*$ for some $C<\infty$ so that the least favorable submodel preserves the bound on the sectional variation norm.

We define
\begin{eqnarray*}
\epsilon_n^{\#}&=&\arg\min_{\epsilon} P_n^{\#}L_1(Q_{n,\epsilon}^{\#})\\
\tilde{\epsilon}_n^{\#}&=&\arg\min_{\epsilon}P_n L_1(Q_{n,\epsilon}^{\#}.
\end{eqnarray*}
Under a weak regularity condition, we have $\mid \epsilon_n^{\#}-\tilde{\epsilon}_n^{\#}\mid =O_P(n^{-1/2}$.
Specifically, this can be shown as follows.
\begin{eqnarray*}
0&\leq & P_n L_1(Q_{n,\epsilon_n^{\#}}^{\#})-P_nL_1(Q_{n,\tilde{\epsilon}_n^{\#}}^{\#})\\
&=& (P_n-P_n^{\#})L_1(Q_{n,\epsilon_n^{\#}}^{\#},Q_{n,\tilde{\epsilon}_n^{\#}}^{\#})\\
&&+ P_n^{\#}L_1(Q_{n,\epsilon_n^{\#}}^{\#},Q_{n,\tilde{\epsilon}_n^{\#}}^{\#})\\
&\leq &-(P_n^{\#}-P_n)L_1(Q_{n,\epsilon_n^{\#}}^{\#},Q_{n,\tilde{\epsilon}_n^{\#}}^{\#})\\
\end{eqnarray*}
The last term is a bootstrapped empirical process which is thus $O_P(n^{-1/2})$. 
An exact first order Tailor expansion at $\tilde{\epsilon}_n^{\#}$ allows us to write the last term as a $(P_n^{\#}-P_n)f_n^{\#}(\epsilon_n^{\#}-\tilde{\epsilon}_n^{\#})$.
A second order Tailor expansion at $\tilde{\epsilon}_n^{\#}$ of the left-hand side of this inequality shows that the left-hand side is a quadratic term behaving as $(\epsilon_n^{\#}-\tilde{\epsilon}_n^{\#})^2$.
Since $(P_n^{\#}-P_n)f_n^{\#}=O_P(n^{-1/2})$, this proves that indeed $\mid \epsilon_n^{\#}-\tilde{\epsilon}_n^{\#}\mid =O_P(n^{-1/2})$.

Let $\epsilon_{0,n}^{\#}=\arg\min_{\epsilon}P_0 L_1(Q_{n,\epsilon}^{\#})$.
Under a weak regularity condition, we have $\tilde{\epsilon}_n^{\#}-\epsilon_{0,n}^{\#}=O_P(n^{-1/2})$.
This is shown as follows.
\begin{eqnarray*}
0&\leq& P_0 L_1(Q_{n,\tilde{\epsilon}_n^{\#}}^{\#})-P_0 L_1(Q_{n,\epsilon_{0,n}^{\#}}^{\#})\\
&=&(P_0-P_n)L_1(Q_{n,\tilde{\epsilon}_n^{\#}}^{\#},Q_{n,\epsilon_{0,n}^{\#}}^{\#})\\
&&+P_n L_1(Q_{n,\tilde{\epsilon}_n^{\#}}^{\#},Q_{n,\epsilon_{0,n}^{\#}}^{\#})\\
&\leq&- (P_n-P_0)L_1(Q_{n,\tilde{\epsilon}_n^{\#}}^{\#},Q_{n,\epsilon_{0,n}^{\#}}^{\#}).
\end{eqnarray*}
The last term is an empirical process which is thus $O_P(n^{-1/2})$.
An exact first order Tailor expansion allows us to write the last term as $(P_n-P_0)f_n^{\#}(\tilde{\epsilon}_n^{\#}-\epsilon_{0,n}^{\#}$.
A second order Tailor expansion at ${\epsilon}_{0,n}^{\#}$ of the left-hand side of this inequality shows that the left-hand side is a quadratic term behaving as $(\tilde{\epsilon}_n^{\#}-\epsilon_{0,n}^{\#})^2$.
Since $(P_n-P_0)f_n^{\#}=O_P(n^{-1/2})$, this proves that indeed $\mid \tilde{\epsilon}_n^{\#}-\epsilon}_{0,n}^{\#}\mid =O_P(n^{-1/2})$.
Thus, we have now also shown $\mid \epsilon_n^{\#}-\epsilon_{0,n}^{\#}=O_P(n^{-1/2})$.

We can now proceed analyzing $Q_{n,\epsilon_n^{\#}}^{\#}$ as follows.
\begin{eqnarray*}
0&\leq &P_0 L_1(Q_{n,\tilde{\epsilon}_n^{\#}}^{\#})-P_0L_1(Q_0)\\
&=&P_0 L_1(Q_{n,\tilde{\epsilon}_n^{\#}}^{\#},Q_{n,\epsilon_{0,n}^{\#}}^{\#})\\
&&+P_0 L_1(Q_{n,\epsilon_{0,n}^{\#}}^{\#},Q_n^{\#})+P_0 L_1(Q_n^{\#},Q_0)\\
&\leq&P_0 L_1(Q_{n,\tilde{\epsilon}_n^{\#}}^{\#},Q_{n,\epsilon_{0,n}^{\#}}^{\#})\\
&&+P_0 L_1(Q_n^{\#},Q_0)\\
&\leq&
-(P_n-P_0) L_1(Q_{n,\tilde{\epsilon}_n^{\#}}^{\#},Q_{n,\epsilon_{0,n}^{\#}}^{\#})\\
&&+P_0 L_1(Q_n^{\#},Q_0).
\end{eqnarray*}
The first term is an empirical process term that can be represented as $(P_n-P_0)f_n^{\#}(\tilde{\epsilon}_n^{\#}-\epsilon_{0,n}^{\#})$, which is thus $O_P(n^{-1}) by our above result. The second term can be written as $P_0L_1(Q_n^{\#},Q_n)+P_0L_1(Q_n,Q_0)$. We have $P_0 L_1(Q_n,Q_0)=O_P(n^{-1/2-\alpha(d)})$.
We also have 
\[
P_0L_1(Q_n^{\#},Q_n)=-(P_n-P_0)L_1(Q_n^{\#},Q_n)+P_n L_1(Q_n^{\#},Q_n)=(P_n-P_0)L_1(Q_n^{\#},Q_n)+O_P(n^{-1/2-\alpha(d)}).\]
Thus, we have shown
\[P_0 L_1(Q_{n,\tilde{\epsilon}_n^{\#}}^{\#})-P_0L_1(Q_0)=O_P(n^{-1/2-\alpha(d)}).\]
Thus, we have shown $d_{01}(Q_{n,\tilde{\epsilon}_n^{\#}}^{\#},Q_0)=O_P(n^{-1/2-\alpha(d)})$ and $\epsilon_n^{\#}-\tilde{\epsilon}_n^{\#}=O_P(n^{-1/2})$.
Due to equivalence of $d_{01}(Q,Q_0)$ with a square of an $L^2$-norm, this also implies $d_{01}(Q_{n,\epsilon_n^{\#}}^{\#},Q_0)=O_P(n^{-1/2-\alpha(d)})$.

\section{Nonparametric bootstrap to estimate a supremum norm of the upper-bound process.}\label{sectsupupperb}

%Define the process $(X_{I,n}(Q,G):(Q,G)\in {\cal F})$ where ${\cal F}={\cal F}_1\times {\cal F}_2)\[X_{I,n}(Q,G)\equiv n^{1/2}(P_n-P_0)D^*(Q_{\epsilon_n},G) +
%\mid n^{1/2}(P_n-P_0)(D^*(Q_n^*,G_n)-D^*(Q_0,G_0))\mid\\ f(d_{01}(Q_{\epsilon_n},Q_0),d_{02}(G,G_0)). \] A user  might decide to use the slightly simpler stochastic process as a good approximation: \[ X_{I,n,a}(Q,G)=n^{1/2}(P_n-P_0)D^*(Q,G) +
%\mid n^{1/2}(P_n-P_0)(D^*(Q_n^*,G_n)-D^*(Q_0,G_0))\mid\\ f(d_{01}(Q,Q_0),d_{02}(G,G_0)).\] The following lemma is trivially true. \begin{lemma}$ X_{I,n}$ is weakly convergence in $\ell^{\infty}({\cal F})$.The nonparametric bootstrap is consistent for $X_{I,n}$.\end{lemma}

%We can use directly empirical process bound for $d_{01}(Q_n^*,Q_0)$, see lemma preserve we now have. No need to replace $Q_n^*$ by $Q_n$.So we can then get rid of $\sim \leq$ and get true inequalities. we can replace $\epsilon_{0n}$ by $\epsilon_n$ giving the $1/n$ error. So that is perfect.This will be much cleaner.

  By Lemma \ref{lemmathalmle} we have ${\bf d}_{01}(Q_n^*,Q_0)\leq -(P_n-P_0){\bf L}_1(Q_n^*,Q_0)+O_P(n^{-1})$ and ${\bf d}_{02}(G_n,G_0)\leq -(P_n-P_0){\bf L}_2(G_n,G_0)$.
 % Since $d_{01}(Q_n^*,Q_0)$ behaves at least as well as  $d_{01}(Q_n,Q_0)$ and is of the same order, we suggest using the same bound for $d_{01}(Q_n^*,Q_0)$. By the same argument, replacing $(P_n-P_0)D^*(Q_n^*,G_n)$ by $(P_n-P_0)D^*(Q_n,G_n)$ should also not be a problem for preserving the conservative nature of our bound. 
  Applying these two upper bounds for ${\bf d}_{01}(Q_n^*,Q_0)$ and ${\bf d}_{02}(G_n,G_0)$ to our upper bound for the second order remainder yields the following conservative bound:
\begin{eqnarray*}
 n^{1/2}\mid \Psi(Q_n^*)-\Psi(Q_0)\mid& \leq & \mid  n^{1/2}(P_n-P_0)D^*(Q_n^*,G_n) \mid \\
 &&\hspace*{-4cm}
 +
%\mid n^{1/2}(P_n-P_0)(D^*(Q_n^*,G_n)-D^*(Q_0,G_0))\mid\\
 f(\sqrt{\mid n^{1/2}(P_n-P_0){\bf L}_1(Q_n^*,Q_0)\mid},\sqrt{ \mid n^{1/2}(P_n-P_0){\bf L}_2(G_n,G_0)\mid})\mid +O_P(n^{-1/2})+n^{1/2}r_n
\end{eqnarray*}
%We use the notation $\sim\leq$ instead of $\leq$ since it is formally known to hold up till the 2 substitutions of $Q_n$ for $Q_n^*$ mentioned above.

Define the following process $X_n=(X_n(Q,G): (Q,G)\in {\cal F})$:
\[
X_n(Q,G)=\mid  n^{1/2}(P_n-P_0)D^*(Q,G) \mid +
%\mid n^{1/2}(P_n-P_0)(D^*(Q_n^*,G_n)-D^*(Q_0,G_0))\mid\\
 f(\mid n^{1/2}(P_n-P_0){\bf L}_1(Q,Q_0)\mid, \mid n^{1/2}(P_n-P_0){\bf L}_2(G,G_0)\mid)\mid .\]
 Thus, we can state that \[
 \mid n^{1/2}(\psi_n^*-\psi_0)\mid \leq \mid X_n(Q_n^*,G_n)\mid +O_P(n^{-1/2})+n^{1/2}\mid P_n D^*(Q_n^*,G_n)\mid.\]
 Let $\tilde{r}_n=O_P(n^{-1/2})+r_n$, and let's assume that $\tilde{r}_n$ is negligible relative to $X_n(Q_n^*,G_n)$ so that we can ignore this term.
 Then, it remains to upper bound $X_n(Q_n^*,G_n)$.
 This suggests the following method for inference:
 \begin{itemize}
 \item For user supplied $\alpha_n=(\alpha_{1n},\alpha_{2n})$, determine an $x_n=(x_{1n},x_{2n})$  so that $P(d_{01}(Q_n^*,Q_0)>x_{1n})\leq \alpha_{1n}$ and $P(d_{02}(G_n,G_0)>x_{2n})\leq \alpha_{2n}$.
  \item Define
 \[ {\cal F}(x_n)=\{(Q,G)\in {\cal F}: d_{01}(Q,Q_0)<x_{1n},d_{02}(G,G_0)<x_{2n}\},\]
 and note that $P((Q_n,G_n)\in {\cal F}(x_n))\geq 1-\bar{\alpha}_n$, where $\bar{\alpha}_n\equiv \alpha_{1n}+\alpha_{2n}$.
 \item We have 
 \[
P(\mid X_n(Q_n^*,G_n)\mid > x)\leq  P(\pl X_n\pl_{{\cal F}(x_n)}>x)+\bar{\alpha}_n ,\]
where $\pl X\pl_{{\cal F}}=\sup_{f\in {\cal F}}\mid X(f)\mid$.
Let 
\[
F_{n,x_1}(x)=P(\pl  X_n \pl_{{\cal F}(x_1)} \leq x),\]
and
\[
q_{n,0.95}=F_{n,x_n}^{-1}(0.95+\bar{\alpha}_n) .\]
If $\tilde{r}_n=0$, then  $\Psi(Q_n^*)\pm q_{n,0.95}/n^{1/2}$ contains $\psi_0$ with probability at least $0.95$.
\item Let $X_n^{\#}$ be the nonparametric bootstrap estimate of $X_n$:
\begin{eqnarray*}
X_n^{\#}(Q,G)&=&\mid  n^{1/2}(P_n^{\#}-P_n)D^*(Q,G) \mid \\
&&\hspace*{-2cm} +
%\mid n^{1/2}(P_n-P_0)(D^*(Q_n^*,G_n)-D^*(Q_0,G_0))\mid\\
 f(\mid n^{1/2}(P_n^{\#}-P_n){\bf L}_1(Q,Q_n)\mid, \mid n^{1/2}(P_n^{\#}-P_n){\bf L}_2(G,G_n)\mid) .\end{eqnarray*}
 \item Let $x_n^{\#}$ be an estimator of $x_n$ using the nonparametric bootstrap. A highly conservative method is presented below, but one could also use
 the conservative sampling distributions $n^{1/2}(P_n^{\#}-P_n)L_1(Q_n^{\#*},Q_n)$ for $d_{01}(Q_n^*,Q_0)$ and $n^{1/2}(P_n^{\#}-P_n)L_2(G_n^{\#},G_n)$ for $d_{02}(G_n,G_0)$. 
%\item We use $\pl  X_n^{\#}\pl_{{\cal F}(x_n)}$ as a conservative sampling distribution estimator of the sampling distribution of $\mid n^{1/2}(\psi_n^*-\psi_0)\mid$.
\item Let  \[ {\cal F}_n(x_n^{\#})=\{(Q,G)\in {\cal F}: d_{n1}(Q,Q_n)<x_{1n}^{\#},d_{n2}(G,G_n)<x_{2n}^{\#}\}\] be the nonparametric bootstrap version of ${\cal F}(x_n)$.
Let 
\[
F_{n,x_1}^{\#}(x)=P(\pl  X_n^{\#} \pl_{{\cal F}_n(x_1)} \leq x\mid (P_n:n\geq 1)).\]
Let 
\[
q_{n,0.95}^{\#}=F_{n,x_n^{\#}}^{\#-1}(0.95+\bar{\alpha}_n) .\]
\item The proposed 0.95-confidence interval is given by:
\[
\psi_n^*\pm q_{n,0.95}^{\#}/n^{1/2} .\]
\end{itemize}
{\bf Method for determining $x_n$:}
In order to implement the above confidence interval we  need to derive a method for determining $x_n$ and its bootstrap version $x_n^{\#}$.
We will now present a conservative method for estimation of $x_n$.
By our integration by parts lemma, we have
\begin{eqnarray*}
d_{01}(Q_n^*,Q_0)&\leq & \pl \bar{P}_n-\bar{P}_0\pl_{\infty}\pl L_1(Q_n^*,Q_0)\pl_v^* +O_P(n^{-1}) \\
&\leq & 2M_1\pl \bar{P}_n-\bar{P}_0\pl_{\infty},\\
d_{02}(G_n,G_0)&\leq &\pl \bar{P}_n-\bar{P}_0\pl_{\infty}\pl L_2(G_n,G_0)\pl_v^* \\
&\leq& 2M_2\pl \bar{P}_n-\bar{P}_0\pl_{\infty}.
\end{eqnarray*}
Let  $T_{n}(x)\equiv P(\pl n^{1/2}(\bar{P}_n-\bar{P}_0)\pl_{\infty}>x)$ so that
$P(d_{01}(Q_n^*,Q_0)>x)\leq T_n( 0.5 xn^{1/2}/M_1)$.
Given $\alpha_{1n},\alpha_{2n}$ we can select $x_{1n}=2M_1n^{-1/2}T_n^{-1}(\alpha_{1n})$ and $x_{2n}=2M_2n^{-1/2}T_n^{-1}(\alpha_{2n})$.
Then, we have that $P(d_{01}(Q_n^*,Q_0)>x_{1n})\leq \alpha_{1n}$ and $P(d_{02}(G_n,G_0)>x_{2n})\leq \alpha_{2n}$.
We also know from empirical process theory that the supremum norm of $n^{1/2}(\bar{P}_n-\bar{P}_0)$ has an exponential tail $\exp(-C x)$ so that
$T_n^{-1}(\alpha_{1n})$ behaves as $\log \alpha_{1n}^{-1}$, and the same applies to $T_n^{-1}(\alpha_{2n})$. This shows that one can select $\alpha_{1n}$ and $\alpha_{2n}$ as numbers that converge to zero at a polynomial rate (e.g. $\alpha_{1n}=n^{-1}$), while still preserving that $\max(x_{1n},x_{2n})\rightarrow 0$ at rate $\log n/n^{1/2}$. 
Since $n^{1/2}(\bar{P}_n-\bar{P}_0)$ is an empirical process indexed by a class of indicators, we can consistently and robustly estimate the distribution of $\pl n^{1/2}(\bar{P}_n-\bar{P}_0)\pl_{\infty}$  with the nonparametric bootstrap \citep{vanderVaart&Wellner96}, which, for completeness,  is  stated in the following lemma.
\begin{lemma}
We have that (uniformly in $x$) $T_{n}(x)\rightarrow T_0(x)$, where $T_0(x)=P(\pl \bar{X}_0\pl_{\infty}>x)$, and 
$\bar{X}_0$ is the limit Gaussian process of $\bar{X}_n=n^{1/2}(\bar{P}_n-\bar{P}_0)$.
We have
\begin{eqnarray*}
P(n^{1/2}d_{01}(Q_n^*,Q_0)>x)&\leq& T_{n}(0.5n^{1/2}x/M_1)\\
P(n^{1/2}d_{02}(G_n,G_0)>x)&\leq & T_{n}(0.5n^{1/2}x/M_2).
\end{eqnarray*}
Let $T_n^{\#}(x)=P(\pl n^{1/2}(\bar{P}_n^{\#}-\bar{P}_n)\pl_{\infty}>x\mid (P_n:n\geq 1))$. Then, uniformly in $x$,
$T_n^{\#}(x)\rightarrow T_0(x)$ as $n\rightarrow\infty$.
\end{lemma}
We estimate $x_n$ with its nonparametric bootstrap analogue: $x_{1n}^{\#}=2M_1 n^{-1/2}T_n^{\#-1}(\alpha_{1n})$ and $x_{2n}^{\#}=2M_2n^{-1/2}T_n^{\#-1}(\alpha_{2n})$.
%Now optimize w.r.t. choice $x_n$
%Let $T_n^{\#}$ be the estimator of the survivor function $T_{0,n}$ of $\pl n^{1/2}(\bar{P}_n-\bar{P}_0)\pl_{\infty}$ based on the nonparametric bootstrap. 

We note that our nonparametric bootstrap estimator of the sampling distribution of $X_n$ and $x_n$ only relies on how well the nonparametric bootstrapped empirical process indexed by Donsker class (functions with uniformly bounded sectional variation norm) and class of indicators approximates the sampling distribution of the empirical process. Therefore, the asymptotic consistency of this nonparametric bootstrap method  follows straightforwardly from the asymptotic consistency of the nonparametric bootstrap for these empirical processes. This is presented in the following theorem. 

 \begin{theorem}
 Consider definitions $X_n$,
 $x_{1n}=2M_1n^{-1/2}T_n^{-1}(\alpha_{1n})$ and $x_{2n}=2M_2n^{-1/2}T_n^{-1}(\alpha_{2n})$. 
 Let $\alpha_n$ converge to zero at a rate $n^{-p}$ for some finite $p$. Then, $x_n$ converges to zero at rate $\log n/n^{1/2}$.
 
{\bf Finite sample oracle confidence interval:} We have
 \[
 \mid n^{1/2}(\psi_n^*-\psi_0)\mid \leq \mid X_n(Q_n^*,G_n)\mid +\tilde{r}_n,\]
 and
 \[
P(\mid X_n(Q_n^*,G_n)\mid > x)\leq  P(\pl X_n\pl_{{\cal F}(x_n)}>x)+\bar{\alpha}_n .\]
Let 
\[
F_{n,x_1}(x)=P(\pl  X_n \pl_{{\cal F}(x_1)} \leq x),\]
and
\[
q_{n,0.95}=F_{n,x_n}^{-1}(0.95+\bar{\alpha}_n) .\]
Then, if $\tilde{r}_n=0$, then  $\Psi(Q_n^*)\pm q_{n,0.95}/n^{1/2}$ contains $\psi_0$ with probability at least $0.95$. 

{\bf Weak convergence of process $X_n$:}
  Let $Z_n$ be the empirical process $n^{1/2}(P_n-P_0)$ indexed by the class of functions 
 \begin{equation}\label{calf1}
 {\cal F}_1\equiv \{D^*(Q,G),L_1(Q,Q_0),L_2(G,G_0): (Q,G)\in {\cal F}\}.
 \end{equation}
  $X_n$ is a continuous function of $Z_n$:
\[
X_n(Q,G)=g(Z_n)\equiv \mid Z_n(D^*(Q,G))\mid +f(\mid Z_n(L_1(Q,Q_0))\mid,\mid Z_n(L_2(G,G_0))\mid) .\]
We know that $Z_n\Rightarrow_d Z_0$ for a Gaussian process in $\ell^{\infty}({\cal F}_1)$.
The continuous mapping theorem shows that $X_n\Rightarrow_d X_0=g(Z_0)$ , where 
$X_0$ is a simple function of $Z_0$ defined by
\[
X_0(Q,G)= \mid Z_0(D^*(Q,G))\mid +f( \mid Z_0(L_1(Q,Q_0))\mid, \mid Z_0(L_2(G,G_0))\mid) .\] 
Therefore, $\pl X_n\pl_{{\cal F}(x)}\Rightarrow \pl X_0\pl_{{\cal F}(x)}$, uniformly in $x$.
In particular, uniformly in $x$
\[
P(\pl X_n\pl_{{\cal F}(x_n)}>x)\rightarrow P(N(0,\sigma^2_0)>x).\]

{\bf Weak convergence of nonparametric bootstrap process $X_n^{\#}$:}
Let $X_n^{\#}$, $x_n^{\#}$, ${\cal F}_n(x_n^{\#})$ be the nonparametric bootstrap version of $X_n$, $x_n$ and ${\cal F}(x_n)$ defined above.
 We have that uniformly in $x$,  conditional on $(P_n:n\geq 1)$, $\pl X_n^{\#}\pl_{{\cal F}(x)}\Rightarrow_d \pl X_0\pl_{{\cal F}(x)}$.
 In particular,
 \[
 P(\pl X_n^{\#}\pl_{{\cal F}(x_n^{\#})}>x\mid (P_n:n\geq 1))+\bar{\alpha}_n\rightarrow P(\mid N(0,\sigma^2_0)\mid >x).\]
 
 {\bf Nonparametric bootstrap estimate of finite sample confidence interval and its asymptotic consistency:}
 Let 
\[
F_{n,x_1}^{\#}(x)=P(\pl  X_n^{\#} \pl_{{\cal F}_n(x_1)} \leq x\mid (P_n:n\geq 1)).\,\]
and
\[
q_{n,0.95}^{\#}=F_{n,x_n^{\#}}^{\#-1}(0.95+\bar{\alpha}_n) .\]

 Then,  $q_{0.95,n}^{\#}(x_n)\rightarrow 1.96$ so that the confidence interval $\psi_n^*\pm q_{0.95,n}^{\#}/n^{1/2}$ is an asymptotic $0.95$-confidence interval.
 \end{theorem}

The width of this proposed confidence interval is a function of the user supplied $\alpha_n=(\alpha_{1n},\alpha_{2n})$. To remove this choice from consideration, one might determine the $\alpha_n$ that minimizes $q_{n,0.95}^{\#}=F_{n,x_n^{\#}}^{\#-1}(0.95+\bar{\alpha}_n) $, where we note that $x_n^{\#}$ depends on $(\alpha_{1n},\alpha_{2n})$.

%The optimal choice $x_n$ minimizing the width of the confidence interval would thus be given by:\[x_n^*\equiv \arg\min_{x}F_{x,n}^{\#,-1}(0.95+(T_{n}^{\#}(x_{1}/M_1)+T_{n}^{\#}(x_{2}/M_2)) ).\]It seems reasonable to set $x_1=c$ and $x_2=c M_2/M_1$ so that $T_{n}^{\#}(x_1/M_1)=T_{n}^{\#}(x_2/M_2)$.Then, the optimal $c$ is given by\[c_n^*\equiv  \arg\min_{c}S_{x(c),n}^{\#,-1}(0.05-2T_{n}^{\#}(c/M_1) ) ,\]where $x(c)=(c,c M_2/M_1)$.

\subsection{Practical implementation}
The implementation of this method requires determining a supremum 
 $\sup_{f\in {\cal F}_n(x_n^{\#})}\mid X_n^{\#}(f)\mid$ of the bootstrapped process $X_n^{\#}$ over $(Q,G) $ in the $x_n^{\#}$-neighborhood
 ${\cal F}_n(x_n^{\#})$  of 
 $(Q_n,G_n)$. It appears reasonable to assume that the supremum will be attained at the edge of ${\cal F}_n(x_n^{\#})$.
  One might aim to approximate this supremum by randomly sampling elements $Q$ and $G$ on the $x_n$-edge of this neighborhood.
 For example, suppose that $d_{n1}(Q,Q_n)=\pl Q-Q_n\pl^2$ is an $L^2$-norm. 
 Suppose we determine a scheme that allows us to sample functions $e$ such that $\pl e\pl^2=x_{1n}^{\#}$. Each such a draw determines a draw $Q=Q_n+e$.
 Similarly, one samples $G=G_n+e$ resulting in a sample $f_1,\ldots,f_J$ of size $J$ on the $x_n$-edge of ${\cal F}_n(x_n^{\#})$.
 The maximum  $\max_j \mid X_n^{\#}(f_j)\mid$ provides then an approximation of the desired supremum $\sup_{f\in {\cal F}_n(x_n^{\#})}\mid X_n^{\#}(f)\mid$.
 Implementation of the supremum $\pl n^{1/2}(\bar{P}_n^{\#}-\bar{P}_n)\pl_{\infty}$ for the sake of determining $x_n^{\#}$ is significantly easier but could also be carried out by taking a random sample from its domain $[0,\tau]$.
 The other components of this method are straightforward to implement.
