# Supplementary material for: Nonparametric Bootstrap Inference for the Targeted Highly Adaptive LASSO Estimator
Source: arXiv:1905.10299 source file (2020-02-07)
Supplement: Supplementary file 2 [file appendix.tex]

\section*{Appendix.}

%Check that results are not only for $d_{01}$ but also for ${\bf d}_{01}$ but now in terms of vector ${\bf L}_1$. Same for $d_{02}$. State that also in lemma.

\section{Proof that the one-step TMLE $Q_n^*$ preserves rate of convergence of $Q_n$}\label{AppendixA}
The following lemma establishes that the one-step TMLE $Q_n^*=Q_{n,\epsilon_n}$ preserves the rate of convergence of $Q_n$, where $Q_{\epsilon}$ is a univariate local least favorable submodel through $Q$ at $\epsilon =0$.
Recall the notation $L_1(Q_1,Q_2)=L_1(Q_1)-L_1(Q_2)$.
%We now want show that $d_{01}(Q_n^*,Q_0)$ is close to $d_{01}(Q_n,Q_0)$.
\begin{lemma}\label{lemmathalmle}
Assume $\epsilon\rightarrow L_1(Q_{n,\epsilon})$ be  differentiable with a uniformly bounded derivative on an interval $\epsilon \in (-\delta,\delta)$ for some $\delta>0$.
Define $\epsilon_{0n}=\arg\min_{\epsilon}P_0 L_1(Q_{n,\epsilon})$, $\epsilon_n=\arg\min_{\epsilon}P_n L_1(Q_{n,\epsilon})$, and assume the weak regularity condition
\begin{equation}\label{Qnstarconv}
\epsilon_{0n}=O_P(d_{01}^{1/2}(Q_n,Q_0)).\end{equation}
Then,
\begin{equation}\label{thalmle}
d_{01}(Q_n^*,Q_0)\leq d_{01}(Q_n,Q_0)+O_P(n^{-1/2-\alpha(d)}).\end{equation}
Specifically,
\begin{eqnarray*}
d_{01}(Q_n^*,Q_0)&\leq& d_{01}(Q_n,Q_0)
%-(P_n-P_0)L_1(Q_{n,\epsilon_{0n}},Q_n)-(P_n-P_0)L_1(Q_n,Q_0)\\&=&-(P_n-P_0)\{L_1(Q_{n,\epsilon_{0n}},Q_n)+L_1(Q_n,Q_0)\}\\
%&=&
-(P_n-P_0)L_1(Q_{n,\epsilon_{0n}},Q_0) .
\end{eqnarray*}
%Under a weak regularity condition, we have $\epsilon_n-\epsilon_{0n}=O_P(n^{-1/2})$.Then,\[d_{01}(Q_n^*,Q_0)\leq -(P_n-P_0)L_1(Q_n^*,Q_0)+O_P(n^{-1}).\]
\end{lemma}
This also proves that the $K$-th step TMLE using a {\em finite} $K$ (uniform in $n$) number of iterations satisfies $d_{01}(Q_n^*,Q_0)\leq d_{01}(Q_n,Q_0)+O_P(n^{-1/2-\alpha(d)})$. So  if $r_n=P_n D^*(Q_{n,\epsilon_n},G_n)$ is not yet $o_P(n^{-1/2})$, then  one should consider  a $K$-th step  TMLE to guarantee that $r_n$ is small enough to be neglected (we know that the fully iterated TMLE will solve $P_n D^*(Q_n^*,G_n)=0$, but this one is harder to analyze).
\newline
{\bf Proof of Lemma \ref{lemmathalmle}:}
%Define $\epsilon_{0n}=\arg\min_{\epsilon}P_0 L_1(Q_{n,\epsilon})$.
Using the MLE properties of $\epsilon_{0n}$ and $Q_n$, subsequently, we obtain
\begin{eqnarray*}
P_0L_1(Q_n^*)-P_0L_1(Q_0)&=&\{ P_0L_1(Q_{n,\epsilon_n})-P_0L_1(Q_{n,\epsilon_{0n}})\}
+\{P_0L_1(Q_{n,\epsilon_{0n}})-P_0L_1(Q_n)\}\\
&&+\{P_0L_1(Q_n)-P_0L_1(Q_0)\}\\
&\leq & P_0L_1(Q_{n,\epsilon_{0n}},Q_n) +P_0L_1(Q_n,Q_0)\\
&=&(P_0-P_n)L_1(Q_{n,\epsilon_{0n}},Q_n) +P_n L_1(Q_{n,\epsilon_{0n}},Q_n)+d_{01}(Q_n,Q_0)\\
&\leq &-(P_n-P_0)L_1(Q_{n,\epsilon_{0n}},Q_n)+d_{01}(Q_n,Q_0)\\
%&=&-(P_n-P_0)L_1(Q_{n,\epsilon_{0n}},Q_0).
\end{eqnarray*}
An exact first order Tailor expansion $f(\epsilon_{0n})-f(0)=\frac{d}{d\xi}f(\xi)\epsilon_{0n}$ for a $\xi$ between $0$ and $\epsilon_{0n}$ applied to $f(\epsilon)=L_1(Q_{n,\epsilon})$ yields:
\[
L_1(Q_{n,\epsilon_{0n} })-L_1(Q_{n})=\epsilon_{0n}\frac{d}{d\xi }L_1(Q_{n,\xi} ).\]
Using that $\epsilon_{0n}$ converges as fast to zero as $d_{01}(Q_n,Q_0)$ and that $(P_n-P_0)L_1(Q_{n,\epsilon_{0n}},Q_0)$ is an evaluation of an  empirical process indexed by  the Donsker class of cadlag functions with sectional variation norm bounded by universal $M_1$, we obtain $(P_n-P_0)L_1(Q_{n,\epsilon_{0n}},Q_n)=O_P(n^{-1/2-\alpha(d)})$, analogue to the proof of this rate of convergence for the  HAL-MLE. So we have
\[
d_{01}(Q_n^*,Q_0)\leq d_{01}(Q_n,Q_0)+O_P(n^{-1/2-\alpha(d)}) .\]
%The first inequality in the above derivation yields $d_{01}(Q_n^*,Q_0)\leq P_0 L_1Firstly, note that the last term can be represented as $It remains to prove the last claim. We have \[(P_n-P_0)L_1(Q_{n,\epsilon_{0n}},Q_0)=(P_n-P_0)L_1(Q_{n,\epsilon_{0n}},Q_{n,\epsilon_n})+(P_n-P_0)L_1(Q_n^*,Q_0).\]We can do an exact tailor expansion at $\epsilon_{0n}$ of the first term so that we obtain $(\epsilon_n-\epsilon_{0n})(P_n-P_0)\frac{d}{d\xi}L_1(Q_{n,\xi})$ at $\xi$ between $\epsilon_n$ and $\epsilon_{0n}$. The latter term is $O_P(n^{-1})$.
$\Box$

\section{Asymptotic convergence of bootstrapped HAL-MLE: Proof of Theorem \ref{thnpbootmle}.}\label{AppendixB}

Consider  a given set $A$ of possible values for $(s,u_s)$, where $s$ is a subset of $\{1,\ldots,m\}$ and $u_s$ is a value in $[0_s,\tau_s]$.
Let $D_{m,C^l,C^u}[0,\tau]=\{f\in D[0,\tau]: C_l\leq \pl f\pl_v^*\leq C^u\}$ be the set of $m$-variate real valued cadlag functions on $[0,\tau]$ with sectional variation norm between $C^l$ and $C^u$. Let $C^l<C^u$. Consider the case that the parameter space $Q({\cal M})$ of $Q(P)=\arg\min_{Q\in Q({\cal M})}PL_1(Q)$ is given by
 \begin{equation}\label{B1}
{\cal F}^{np}_A\equiv \{F\in D_{m,C^l,C^u}[0,\tau]: dF_s(u_s)=I_{(s,u_s)\in A}dF_s(u_s)\}.\end{equation}
Here we use the short-hand notation $g(x)=I_{x\in A}g(x)$ to state that $g(x)=0$ for $x\not \in A$.
Recall that each function $F\in D_{m,C^l,C^u}[0,\tau]$ can be represented as $F(x)=F(0)+\sum_{s\subset \{1,\ldots,m\}}\int_{(0_s,x_s]} dF_s(u_s)$, while
$\pl F\pl_v^*=\mid F(0)\mid +\sum_{s\subset\{1,\ldots,m\}}\int_{(0_s,\tau_s]}\mid dF_s(u_s)\mid$.
We also consider the case that the parameter space $Q({\cal M})$ equals
\begin{equation}\label{B2}
{\cal F}^{np+}_A\equiv \{F\in D_{m,C^l,C^u}[0,\tau]: dF_s(u_s)=I_{(s,u_s)\in A}dF_s(u_s),dF_s(u_s)\geq 0,F(0)\geq 0\}.\end{equation}
For this case, we allow that $C^l=C^u$.
If we select $A$ is unrestricted, then ${\cal F}^{np}_A$ is the set of all $m$-variate cadlag functions with sectional variation norm bounded by $(C^l,C^u)$, and
${\cal F}^{np+}_A$ is the set of non-negative monotone functions  with positive total mass between $C^l$ and $C^u$  (i.e.,we obtain a set of  cumulative distributions if $C^l=C^u=1$).
So the set $A$ indicates that $dF_s(u_s)$ is only non-zero for $(s,u_s)\in A$ and thereby restricts the set of possible functions in the parameter space.

In our model defined in Section 2 we assumed that each component of $Q$ and $G$ has its own loss and such a parameter space, and the HAL-MLE can be computed separately for each of these components. Thus, by applying our results below to each component of $Q$ and $G$ separately with $L_1(Q)$ replaced by its loss function, $Q_n$ and $Q_n^{\#}$ replaced by its HAL-MLE and  HAL-MLE applied to bootstrap sample, respectively, one obtains the desired result for each component.

 The next Theorem \ref{ThB} shows that $d_{n1}(Q_n^{\#},Q_n)=P_n \{L_1(Q_n^{\#})-L_1(Q_n)\}$ converges at rate $n^{-1/2-\alpha(d)}$ and that this empirical loss-based dissimilarity $d_{n1}(Q_n^{\#},Q_n)$ dominates a quadratic dissimilarity (making it equally powerful as $d_{01}(Q_n,Q_0)$).

\begin{theorem}\label{ThB}
Recall Definition \ref{defabscont} of $Q\ll Q_n$.
Let $Q_n=\arg\min_{Q\in Q({\cal M}}P_nL_1(Q)$, $Q_n^{\#}=\arg\min_{Q\in Q({\cal M}),Q\ll Q_n}P_n^{\#}L_1(Q)$ be the HAL-MLE and HAL-MLE on the bootstrap sample, respectively, where $Q({\cal M})$ either equals ${\cal F}_A^{np}$ (\ref{B1}) or ${\cal F}_A^{np+}$ (\ref{B2}).
Either assume $\pl Q_n\pl_v^*=C^u$ or assume that $\pl Q_n^{\#}\pl_v^*\leq \pl Q_n\pl_v^*$ (and $\pl Q_n\pl_v^*>C^l$ if $C^l<C^u$), conditional on $(P_n:n\geq 1)$.

Let $P_n R_{2L_1,n}(Q_n^{\#},Q_n)$ be defined by
\[
P_n \{L_1(Q_n^{\#})-L_1(Q_n)\}=P_n \frac{d}{dQ_n}L_1(Q_n)(Q_n^{\#}-Q_n)+P_n R_{2L_1,n}(Q_n^{\#},Q_n).\]
%for some second-order term $R_{2L_1,n}(Q_n^{\#},Q_n)$ involving square differences between $Q_n^{\#}$ and $Q_n$.

We have $P_n\frac{d}{dQ_n}L_1(Q_n)(Q_n^{\#}-Q_n)\geq 0$ so that
\[
d_{n1}(Q_n^{\#},Q_n) \geq P_n R_{2L_1,n}(Q_n^{\#},Q_n).\]
Thus, if
\[
P_n \{L_1(Q_n^{\#})-L_1(Q_n)\}^2\lesssim P_nR_{2L_1,n}(Q_n^{\#},Q_n),\]
then
\begin{equation}\label{b3}
P_n \{L_1(Q_n^{\#})-L_1(Q_n)\}^2\lesssim d_{n1}(Q_n^{\#},Q_n).\end{equation}
Suppose the latter (\ref{b3}) holds.
By Lemma \ref{generalhalmle} below, then
\[ d_{n1}(Q_n^{\#},Q_n)=O_P(n^{-1/2-\alpha(d)}).\]
This, on its turn then  implies
 $P_nR_{2L_1,n}(Q_n^{\#},Q_n)=O_P(n^{-1/2-\alpha(d)})$.
\end{theorem}

In order to provide the reader a concrete example, we provide here the corollary for the squared error loss.
\begin{corollary}
Consider definition and assumptions of Theorem \ref{ThB}.
Suppose that $L_1(Q)(O)=(Y-Q(X))^2$ is the squared error loss.
%The parameter space of $Q$ is given by ${\cal F}_A^{np}$ defined above.
Then,
we have
\[
d_{n1}(Q_n^{\#},Q_n)\geq P_n (Q_n^{\#}-Q_n)^2 .\]
Since  $P_n  \{L_1(Q_n^{\#})-L_1(Q_n)\}^2\lesssim P_n (Q_n^{\#}-Q_n)^2$, this implies
$P_n  \{L_1(Q_n^{\#})-L_1(Q_n)\}^2\lesssim d_{n1}(Q_n^{\#},Q_n)$.
By Lemma \ref{generalhalmle}, this shows
\[
d_{n1}(Q_n^{\#},Q_n)=O_P(n^{-1/2-\alpha(d)}).
\]
This, on its turn then implies  $P_n (Q_n^{\#}-Q_n)^2=O_P(n^{-1/2-\alpha(d)})$.
\end{corollary}

%Note that $Q_n$ is an element of the parameter space over which $Q_n^{\#}$ minimizes its empirical risk.We need to prove that $d_{n1}(Q_n^{\#},Q_n)=P_n \{L_1(Q_n^{\#})-L_1(Q_n)\}$ converges at rate $n^{-1/2-\alpha(d)}$ and that this empirical loss-based dissimilarity $d_{n1}(Q_n^{\#},Q_n)$ dominates a quadratic dissimilarity (making it equally powerful as $d_{01}(Q_n,Q_0)$).

To prove Theorem \ref{ThB}, we first present the following straightforward lemma, which follows immediately by just imitating the proof of the convergence of the HAL-MLE $Q_n$ itself but now under sampling from $P_n$. Here one uses that $P_n^{\#}L_1(Q_n^{\#})-P_n^{\#}L_1(Q_n)\leq 0$, since $Q_n$ is an element of the parameter space over which $Q_n^{\#}$ minimizes $P_n^{\#}L_1(Q)$.

\begin{lemma}\label{generalhalmle}
Consider the above setting.
We have
\begin{eqnarray}
0&\leq & d_{n1}(Q_n^{\#},Q_n)\equiv P_n\{ L_1(Q_n^{\#})-L_1(Q_n)\}\nonumber \\
&=& -(P_n^{\#}-P_n)\{L_1(Q_n^{\#})-L_1(Q_n)\}+P_n^{\#}\{L_1(Q_n^{\#})-L_1(Q_n)\}\nonumber \\
&\leq& -(P_n^{\#}-P_n)\{L_1(Q_n^{\#})-L_1(Q_n)\}.\label{boota}
\end{eqnarray}
%and similarly $d_{n2}(G_n^{\#},G_n)\leq -(P_n^{\#}-P_n)L_2(G_n^{\#},G_n)$.
As a consequence, by empirical process theory \citep{vanderVaart&Wellner11}, we have $d_{n1}(Q_n^{\#},Q_n)=P_n L_1(Q_n^{\#})-P_nL_1(Q_n)$ is $O_P(n^{-1/2})$, and
% and $d_{n2}(G_n^{\#},G_n)=P_n L_2(G_n^{\#})-P_nL_2(G_n)$ are both $O_P(n^{-1/2})$.
%In addition, since $L_1(Q_n^{\#})-L_1(Q_n)$ falls in a uniform Donsker class with probability 1 so that the empirical process is asymptotically equicontinuous, we have that if  $d_{n1}(Q_n^{\#},Q_n)\rightarrow 0$ and $d_{n2}(G_n^{\#},G_n)\rightarrow 0$ implies that $P_n \{L_1(Q_n^{\#})-L_1(Q_n)\}^2\rightarrow 0$ and $P_n \{L_2(G_n^{\#})-L_2(G_n)\}^2\rightarrow 0$, then we have $d_{n1}(Q_n^{\#},Q_n)=o_P(n^{-1/2})$ and $d_{n2}(G_n^{\#},G_n)=o_P(n^{-1/2})$.
if $\pl L_1(Q_n^{\#})-L_1(Q_n)\pl_{P_n}^2\lesssim d_{n1}(Q_n^{\#},Q_n)$, then we have
$d_{n1}(Q_n^{\#},Q_n)=O_P(n^{-1/2-\alpha(d)})$.
% and similarly for $G_n^{\#}$.
\end{lemma}

{\bf Proof of Theorem \ref{ThB}:}
We first prove the results for the general loss function, and subsequently, we will consider the special case that $L_1(Q)$ is the squared error loss.
Consider the  $h$-specific path  \[
Q_{n,\epsilon}^h(x)=(1+\epsilon h(0))Q_n(0)+\sum_s \int_{(0_s,x_s]}(1+\epsilon h_s(u_s)) dQ_{n,s}(u_s))\]
 for $\epsilon \in [0,\delta)$ for some $\delta>0$, where $h$ is uniformly bounded, and,  if $C^l<C^u$,  \[
 r(h,Q_n)\equiv  h(0)\mid Q_n(0)\mid+\sum_s \int_{(0_s,\tau_s]} h_s(u_s)\mid dQ_{n,s}(u_s)\mid \leq 0,\] while if $C^l=C^u$, then $r(h,Q_n)=0$.  Let ${\cal H}=\{h: r(h,Q_n)\leq 0,\pl h\pl_{\infty}<\infty\}$ be the set of possible functions $h$(i.e., functions of $s,u_s$), which defines a collection of paths $\{Q_{n,\epsilon}^h:\epsilon\}$ indexed by $h\in {\cal H}$. Consider a given $h\in {\cal H}$ and let's denote this path with $Q_{n,\epsilon}$, suppressing the dependence on $h$ in the notation.
For $\epsilon\geq 0$ small enough we have $(1+\epsilon h(0))>0$ and $1+\epsilon h_s(u_s)>0$. Thus, for $\epsilon\geq $ small enough we have
\begin{eqnarray*}
\pl Q_{n,\epsilon}\pl_v^*&=&(1+\epsilon h(0))\mid Q_n(0)\mid+\sum_s \int_{(0_s,\tau_s]}(1+\epsilon h_s(u_s))\mid dQ_{n,s}(u_s)\mid \\
&=& \pl Q_n\pl_v^*+\epsilon\left\{ h(0)\mid Q_n(0)\mid+\sum_s \int_{(0_s,\tau_s]}h_s(u_s) \mid dQ_{n,s}(u_s)\mid \right\} \\
&=&\pl Q_n\pl_v^*+\epsilon r(h,Q_n)\\
&\leq & \pl Q_n\pl_v^*,
\end{eqnarray*}
by assumption that $r(h,Q_n)\leq 0$. If $C^l=C^u$ and thus $r(h,Q_n)=0$, then the above shows $\pl Q_{n,\epsilon}\pl_v^*=\pl Q_n\pl_v^*$.
Thus, for a small enough $\delta>0$ $\{Q_{n,\epsilon}:0\leq \epsilon<\delta\}$ represents a path of cadlag functions with sectional variation norm  bounded from below by $C^l$ and smaller than or equal to $\pl Q_n\pl_v^*\leq C^u$. In addition, we have that $dQ_{n,s}(u_s)=0$ implies $(1+\epsilon h_s(u_s))dQ_{n,s}(u_s)=0$ so that the support of $Q_{n,\epsilon}$ is included in the support $A$ of $Q_n$ as defined by ${\cal F}_A^{np}$. Thus, this proves that for $\delta>0$ small enough this path $\{Q_{n,\epsilon}:0\leq \epsilon\leq \delta\}$ is indeed a  submodel of the parameter space of $Q$, defined as ${\cal F}_{A}^{np}$ or ${\cal F}_A^{np+}$.

We also have that
 \[
 Q_{n,\epsilon}-Q_n=\epsilon\left\{ Q_n(0)h(0)+ \sum_s \int_{(0_s,x_s]} h_s(u_s)dQ_{n,s}(u_s)\right\} .\]
 Thus, this path generates a direction $f(h,Q_n)$  at $\epsilon=0$ given by:
 \[
 \frac{d}{d\epsilon}Q_{n,\epsilon}=f(h,Q_n)\equiv Q_n(0)h(0)+ \sum_s \int_{(0_s,x_s]} h_s(u_s)dQ_{n,s}(u_s) .\]
 %Note that $f(h,Q_n)$ represents a difference of two cadlag functions.
 Let ${\cal S}\equiv \{f(h,Q_n): h\in {\cal H}\}$ be the collection of directions generated by our family of paths.
 By definition of the MLE $Q_n$, we also have that $\epsilon \rightarrow P_n L_1(Q_{n,\epsilon})$ is minimal over $[0,\delta)$ at $\epsilon =0$.
This shows that the derivative of $P_n L_1(Q_{n,\epsilon})$ from the right at $\epsilon =0$ is  non-negative:
 \[
 \frac{d}{d\epsilon^+ }P_n L_1(Q_{n,\epsilon })\geq 0\mbox{ at $\epsilon =0$}.\]
 This derivative is given by $P_n \frac{d}{dQ_n}L_1(Q_n)(f(h,Q_n))$, where $d/dQ_nL_1(Q_n)(f(h,Q_n))$ is the directional (Gateaux) derivative of $Q\rightarrow L_1(Q)$ at $Q_n$ in  in direction $f(h,Q_n)$.
  Thus for each $h\in {\cal H}$, we have
\[
P_n \frac{d}{dQ_n}L_1(Q_n)(f(h,Q_n)) \geq 0 .\]
Suppose that
\begin{equation}\label{keya1}
Q_n^{\#}-Q_n\in {\cal S}=\{f(h,Q_n):h\in {\cal H}\}.\end{equation}
Then, we have
\[
P_n \frac{d}{dQ_n}L_1(Q_n)(Q_n^{\#}-Q_n)\geq 0.\]
Combined with the stated second-order Tailor expansion of $P_n L_1(Q)$ at $Q=Q_n$ with exact second-order remainder  $P_nR_{2L_1,n}(Q_n^{\#},Q_n)$, this proves
%\[P_n \{L_1(Q_n^{\#})-L_1(Q_n)\}=P_n \frac{d}{dQ_n}L_1(Q%_n)(Q_n^{\#}-Q_n)+R_2(Q_n^{\#},Q_n)\]for some second-order remainder involving square differences between $Q_n^{\#}$ and $Q_n$. Then,
\[
P_n\{L_1(Q_n^{\#})-L_1(Q_n)\}\geq P_nR_{2L_1,n}(Q_n^{\#},Q_n).\]
%Applying empirical process theory \citep{vanderVaart&Wellner11} to (\ref{boota}) now proves all statements of Lemma \ref{bootstrapHALMLEstructure}.
Thus it remains to show (\ref{keya1}).

% Since $\pl Q_n^\#}\pl_v^*=\pl Q_n\pl_v^*=M$ will both achieve the maximal allowed variation norm, and  $Q_{n,s}^{\#}\ll Q_{n,s}$ for all subset $s$ (i.e., the support of $Q_{n,s}^{\#}$ is a subset of the support of $Q_{n,s}$ due to the support of $P_n^{\#}$ being  a subset of support of $P_n$), one would generally expect that indeed this difference $Q_n^{\#}-Q_n$ is included in ${\cal S}$.
In order to prove (\ref{keya1}), let's solve explicitly for $h$ so that $Q_n^{\#}-Q_n=f(h,Q_n)$ and then verify that $h\in {\cal H}$ satisfies its assumed constraints (i.e., $r(h,Q_n)\leq 0$ if $C^l<C^u$ or $r(h,Q_n)=0$ if $C^l=C^u$,  and $h$ is uniformly bounded).
We have
\begin{eqnarray*}
Q_n^{\#}-Q_n&=&Q_n^{\#}(0)-Q_n(0)+\sum_s\int_{(0_s,x_s]} d(Q_{n,s}^{\#}-dQ_{n,s})(u_s)\\
&=& Q_n^{\#}(0)-Q_n(0)+\sum_s \int_{(0_s,x_s]} \frac{d(Q_{n,s}^{\#}-dQ_{n,s})}{dQ_{n,s}} dQ_{n,s}(u_s),
\end{eqnarray*}
where we used that $Q_{n,s}^{\#}\ll Q_{n,s}$ for each subset $s$.
%since the support of the bootstrap sample is  a subset of  the support $\{O_1,\ldots,O_n\}$ of $P_n$.
Let $h(Q_n^{\#},Q_n)$ be defined by
\begin{eqnarray*}
h(Q_n^{\#},Q_n)(0)&=&(Q_n^{\#}(0)-Q_n(0))/Q_n(0)\\
h_s(Q_n^{\#},Q_n)&=&\frac{d(Q_{n,s}^{\#}-dQ_{n,s})}{dQ_{n,s}}\mbox{ for all subsets $s$} .
\end{eqnarray*}
For this choice $h(Q_n^{\#},Q_n)$, we have $f(h,Q_n)=Q_n^{\#}-Q_n$.
First, consider the case $Q({\cal M})={\cal F}_A^{np}$ or $Q({\cal M})={\cal F}_A^{np+}$, but$C^l<C^u$.
We now need to verify if  $r(h,Q_n)\leq 0$ for this choice $h=h(Q_n^{\#},Q_n)$.
We have
\begin{eqnarray*}
r(h,Q_n)&=&\frac{Q_n^{\#}(0)-Q_n(0)}{Q_n(0)}\mid Q_n(0)\mid+\sum_s\int_{(0_s,\tau_s]}\frac{dQ_{n,s}^{\#}-dQ_{n,s}}{dQ_{n,s}}\mid dQ_{n,s}\mid\\
&=&I(Q_n(0)>0)\{Q_n^{\#}(0)-Q_n(0)\}+I(Q_n(0)\leq 0)\{Q_n(0)-Q_n^{\#}(0)\}\\
&&+\sum_s\int_{(0_s,\tau_s]}I(dQ_{n,s}\geq 0) d(Q_{n,s}^{\#}-dQ_{n,s})\\
&&+\sum_s\int_{(0_s,\tau_s]} I(dQ_{n,s}<0)d(Q_{n,s}-Q_{n,s}^{\#})\\
&=&-\pl Q_n\pl_v^*+Q_n^{\#}(0)\{ I(Q_n(0)>0)-I(Q_n(0)\leq 0)\} \\
&&+\sum_s \int_{(0_s,\tau_s]}\{I(dQ_{n,s}\geq 0) -I(dQ_{n,s}\leq 0\} dQ_{n,s}^{\#}\\
&\leq&-\pl Q_n\pl_v^*+\mid Q_n^{\#}(0)\mid +\sum_s\int_{(0_s,\tau_s]} \mid dQ_{n,s}^{\#}(u_s)\mid \\
&=&-\pl Q_n\pl_v^*+\pl Q_n^{\#}\pl_v^*\\
&\leq &0,
\end{eqnarray*}
since $\pl Q_n^{\#}\pl_v^*\leq \pl Q_n\pl_v^*$, by assumption.
Thus, this proves that indeed $r(h,Q_n)\leq 0$ and thus that $Q_n^{\#}-Q_n\in {\cal S}$.
Consider now the case that $Q({\cal M})={\cal F}_A^{np+}$ {\em and } $C^l=C^u$. Then $\pl Q_n\pl_v^*=\pl Q_n^{\#}\pl_v^*=C^u$. We now need to show that $r(h,Q_n)=0$ for this choice $h=h(Q_n^{\#},Q_n)$. We now use the same three equalities as above, but now use that $dQ_{n,s}(u_s)\geq 0$ and $Q_n(0)\geq 0$, by definition of ${\cal F}_A^{np+}$, which then shows $r(h,Q_n)=0$.
This proves (\ref{keya1}) and thereby Theorem \ref{ThB}.

Consider  now the squared error loss $L_1(Q)=(Y-Q(X))^2$. Then,
\begin{eqnarray*}
d_{n1}(Q_n^{\#},Q_n)&=&\frac{1}{n}\sum_i \{2Y_iQ_n(X_i)-2Y_i Q_n^{\#}(X_i)+Q_n^{\#2}(X_i)-Q_n^2(X_i)\}\\
&=& \frac{1}{n}\sum_i\{2  (Q_n-Q_n^{\#})(X_i)  Y_i+Q_n^{\#2}(X_i)-Q_n^2(X_i)\}\\
&=&\frac{1}{n}\sum_i \{2(Q_n-Q_n^{\#})(X_i)(Y_i-Q_n(X_i))\\
&&\hfill +2(Q_n-Q_n^{\#})Q_n(X_i)+Q_n^{\#2}(X_i)-Q_n^2(X_i)\}\\
&=&\frac{1}{n}\sum_i 2(Q_n-Q_n^{\#})(X_i)(Y_i-Q_n(X_i))+\frac{1}{n}\sum_i (Q_n-Q_n^{\#})^2(X_i).\end{eqnarray*}
Note that the first term corresponds with $P_n\frac{d}{dQ_n}L_1(Q_n)(Q_n^{\#}-Q_n)$ and the second-order term with $P_nR_{2L_1,n}(Q_n^{\#},Q_n)$, where
$R_{2L_1,n}(Q_n^{\#},Q_n)=(Q_n^{\#}-Q_n)^2$.
We want to show that $ \frac{1}{n}\sum_i 2(Q_n-Q_n^{\#})(X_i)(Y_i-Q_n(X_i))\geq 0$.
The general equation above $P_n \frac{d}{dQ_n}L_1(Q_n)(f(h,Q_n)) \geq 0$ corresponds for the squared error loss with:
\[
-2 \frac{1}{n}\sum_i f(h,Q_n)(Y_i-Q_n(X_i)) \geq 0.\]
As we showed in general above  we have that $f(h,Q_n)$ can be chosen to be equal to $Q_n^{\#}-Q_n$.
So this proves that $n^{-1}\sum_i(Q_n^{\#}-Q_n)(X_i)(Y_i-Q_n(X_i))\leq 0$. This proves the desired result for the squared error loss.
Specifically,
\[
d_{n1}(Q_n^{\#},Q_n)\geq P_n (Q_n-Q_n^{\#})^2.\]
Clearly, $P_n  \{L_1(Q_n^{\#})-L_1(Q_n)\}^2\leq C P_n (Q_n^{\#}-Q_n)^2\leq Cd_{n1}(Q_n^{\#},Q_n)$ for some $C<\infty$.
Lemma \ref{generalhalmle} now shows \[
d_{n1}(Q_n^{\#},Q_n)=O_P(n^{-1/2-\alpha(d)}).\]
This completes the proof of Theorem \ref{ThB} and its corollary for the squared error loss. $\Box$

We now prove Lemma \ref{lemmadndo}.
\begin{lemma}\label{dndo}
%The question is then if the desired convergence in this $L^2(P_n)$-norm also implies this same rate of convergence w.r.t. $L^2(P_0)$-norm.
Suppose that $\int f^2_n dP_n=O_P(n^{-1/2-\alpha(d)})$ and we know that $\pl f_n\pl_v^*<M$ for some $M<\infty$.
Then $\int f_n^2dP_0=O_P(n^{-1/2-\alpha(d)})$.
\end{lemma}
{\bf Proof:}
We have
\begin{eqnarray*}
\int f_n^2 dP_0&=&-\int f_n^2d(P_n-P_0)+\int f_n^2 dP_n\\
&=&-\int f_n^2 d(P_n-P_0)+O_P(n^{-1/2-\alpha(d)}).
\end{eqnarray*}
We have $\int f_n^2 d(P_n-P_0)=O_P(n^{-1/2})$.
This proves that $\int f_n^2 dP_0=O_P(n^{-1/2})$. By asymptotic equicontinuity of the empirical process indexed by cadlag functions with uniformly bounded sectional variation norm, it follows now also that $\int f_n^2 d(P_n-P_0)=O_P(n^{-1/2-\alpha(d)})$. Thus, this proves that indeed
that $\int f_n^2 dP_0=O_P(n^{-1/2-\alpha(d)})$ follows from $\int f_n^2dP_n=O_P(n^{-1/2-\alpha(d)})$.
$\Box$

\section{Preservation of rate of one-step TMLE $Q_{n,\epsilon_n}$ under sampling from $P_n$}\label{AppendixC}
%In our theorem we just assumed $\epsilon_n^{\#2}=O_P(n^{-1/2-\alpha(d)})$.Below, we show that under regularity conditions, indeed $d_{01}(Q_{n,\epsilon_n^{\#}}^{\#},Q_0)=O_P(n^{-1/2-\alpha(d)})$.
As the following proof demonstrates, if $\epsilon\rightarrow  L_1(Q_{\epsilon})$ is twice differentiable, and the minima $\tilde{\epsilon}_n^{\#}$ of $P_n L_1(Q_{n,\epsilon}^{\#})$ and $\epsilon_{0,n}^{\#}$ of $P_0L_1(Q_{n,\epsilon}^{\#})$ are interior minima with derivative equal to zero, then
$d_{01}(Q_{n,\epsilon_n^{\#}}^{\#},Q_0)=O_P(n^{-1/2-\alpha(d)})$, showing that indeed the one-step TMLE $Q_{n,\epsilon_n}$ also preserves the rate of convergence of the HAL-MLE under sampling from $P_n$.

Recall that $\sup_{\epsilon}\pl Q_{\epsilon}\pl_v^*< C \pl Q\pl_v^*$ for some $C<\infty$ so that the least favorable submodel preserves the bound on the sectional variation norm.

We define
\begin{eqnarray*}
\epsilon_n^{\#}&=&\arg\min_{\epsilon} P_n^{\#}L_1(Q_{n,\epsilon}^{\#})\\
\tilde{\epsilon}_n^{\#}&=&\arg\min_{\epsilon}P_n L_1(Q_{n,\epsilon}^{\#}).
\end{eqnarray*}
Under a weak regularity condition, we have $\mid \epsilon_n^{\#}-\tilde{\epsilon}_n^{\#}\mid =O_P(n^{-1/2})$.
Specifically, this can be shown as follows.
\begin{eqnarray*}
0&\leq & P_n L_1(Q_{n,\epsilon_n^{\#}}^{\#})-P_nL_1(Q_{n,\tilde{\epsilon}_n^{\#}}^{\#})\\
&=& (P_n-P_n^{\#})L_1(Q_{n,\epsilon_n^{\#}}^{\#},Q_{n,\tilde{\epsilon}_n^{\#}}^{\#})\\
&&+ P_n^{\#}L_1(Q_{n,\epsilon_n^{\#}}^{\#},Q_{n,\tilde{\epsilon}_n^{\#}}^{\#})\\
&\leq &-(P_n^{\#}-P_n)L_1(Q_{n,\epsilon_n^{\#}}^{\#},Q_{n,\tilde{\epsilon}_n^{\#}}^{\#}).\\
\end{eqnarray*}
The last term is a bootstrapped empirical process which is thus $O_P(n^{-1/2})$.
An exact first order Tailor expansion at $\tilde{\epsilon}_n^{\#}$ allows us to write the last term as a $(P_n^{\#}-P_n)f_n^{\#}(\epsilon_n^{\#}-\tilde{\epsilon}_n^{\#})$ for a specified function $f_n$.
A second-order Tailor expansion at $\tilde{\epsilon}_n^{\#}$ of the left-hand side of this inequality and using that the first derivative at $\tilde{\epsilon}_n^{\#}$ is zero (since it is a minimum) shows that the left-hand side is a quadratic term behaving as $(\epsilon_n^{\#}-\tilde{\epsilon}_n^{\#})^2$.
Since $(P_n^{\#}-P_n)f_n^{\#}=O_P(n^{-1/2})$, this proves that  $\mid \epsilon_n^{\#}-\tilde{\epsilon}_n^{\#}\mid^2 =O_P(n^{-1/2}\mid \epsilon_n^{\#}-\tilde{\epsilon}_n^{\#}\mid)$, and thus $\mid \epsilon_n^{\#}-\tilde{\epsilon}_n^{\#}\mid =O_P(n^{-1/2})$.

Let $\epsilon_{0,n}^{\#}=\arg\min_{\epsilon}P_0 L_1(Q_{n,\epsilon}^{\#})$.
Under a weak regularity condition, we also have $\tilde{\epsilon}_n^{\#}-\epsilon_{0,n}^{\#}=O_P(n^{-1/2})$.
This is shown similarly:
\begin{eqnarray*}
0&\leq& P_0 L_1(Q_{n,\tilde{\epsilon}_n^{\#}}^{\#})-P_0 L_1(Q_{n,\epsilon_{0,n}^{\#}}^{\#})\\
&=&(P_0-P_n)L_1(Q_{n,\tilde{\epsilon}_n^{\#}}^{\#},Q_{n,\epsilon_{0,n}^{\#}}^{\#})+P_n L_1(Q_{n,\tilde{\epsilon}_n^{\#}}^{\#},Q_{n,\epsilon_{0,n}^{\#}}^{\#})\\
&\leq&- (P_n-P_0)L_1(Q_{n,\tilde{\epsilon}_n^{\#}}^{\#},Q_{n,\epsilon_{0,n}^{\#}}^{\#}).
\end{eqnarray*}
The last term is an empirical process which is thus $O_P(n^{-1/2})$.
An exact first order Tailor expansion allows us to write the last term as $(P_n-P_0)f_n^{\#}(\tilde{\epsilon}_n^{\#}-\epsilon_{0,n}^{\#})$.
A second-order Tailor expansion at ${\epsilon}_{0,n}^{\#}$ of the left-hand side of this inequality and using that the first derivative at the minimum $\epsilon_{0,n}^{\#}$ equals zero shows that the left-hand side is a quadratic term behaving as $(\tilde{\epsilon}_n^{\#}-\epsilon_{0,n}^{\#})^2$.
Since $(P_n-P_0)f_n^{\#}=O_P(n^{-1/2})$, this proves that indeed $\mid \tilde{\epsilon}_n^{\#}-\epsilon_{0,n}^{\#}\mid =O_P(n^{-1/2})$.

%Combining these two $O_P(n^{-1/2})$ bounds implies $\mid \epsilon_n^{\#}-\epsilon_{0,n}^{\#}\mid =O_P(n^{-1/2})$.

We will now bound $d_{01}(Q_{n,\tilde{\epsilon}_n^{\#}}^{\#},Q_0)$, where we use the latter  $\mid \tilde{\epsilon}_n^{\#}-\epsilon_{0,n}^{\#}\mid =O_P(n^{-1/2})$, and, combined with $\epsilon_n^{\#}-\tilde{\epsilon}_n^{\#}=O_P(n^{-1/2})$ this will give the desired result for $d_{01}(Q_{n,\epsilon_n^{\#}}^{\#},Q_0)$.
Using that $\epsilon_{0,n}^{\#}$ minimizes $P_0L_1(Q_{n,\epsilon}^{\#})$ and $\tilde{\epsilon}_n^{\#}$ minimizes $P_n L_1(Q_{n,\epsilon}^{\#})$ provides us with the following two  subsequent inequalities:
\begin{eqnarray*}
0&\leq &P_0 L_1(Q_{n,\tilde{\epsilon}_n^{\#}}^{\#})-P_0L_1(Q_0)\\
&=&P_0 L_1(Q_{n,\tilde{\epsilon}_n^{\#}}^{\#},Q_{n,\epsilon_{0,n}^{\#}}^{\#})\\
&&+P_0 L_1(Q_{n,\epsilon_{0,n}^{\#}}^{\#},Q_n^{\#})+P_0 L_1(Q_n^{\#},Q_0)\\
&\leq&P_0 L_1(Q_{n,\tilde{\epsilon}_n^{\#}}^{\#},Q_{n,\epsilon_{0,n}^{\#}}^{\#})+P_0 L_1(Q_n^{\#},Q_0)\\
&=&
-(P_n-P_0) L_1(Q_{n,\tilde{\epsilon}_n^{\#}}^{\#},Q_{n,\epsilon_{0,n}^{\#}}^{\#})+P_n L_1(Q_{n,\tilde{\epsilon}_n^{\#}}^{\#},Q_{n,\epsilon_{0,n}^{\#}}^{\#})\\
&&+P_0 L_1(Q_n^{\#},Q_0)\\
&\leq & -(P_n-P_0) L_1(Q_{n,\tilde{\epsilon}_n^{\#}}^{\#},Q_{n,\epsilon_{0,n}^{\#}}^{\#})+P_0 L_1(Q_n^{\#},Q_0).\\
\end{eqnarray*}
Using an exact first order Tailor expansion at $\epsilon_{0,n}^{\#}$, the first  empirical process term can be represented as  $(P_n-P_0)f_n^{\#}(\tilde{\epsilon}_n^{\#}-\epsilon_{0,n}^{\#})$, which is thus $O_P(n^{-1})$. The second term can be written as $P_0L_1(Q_n^{\#},Q_n)+P_0L_1(Q_n,Q_0)$. We have $P_0 L_1(Q_n,Q_0)=O_P(n^{-1/2-\alpha(d)})$.
We also have
\begin{eqnarray*}
P_0L_1(Q_n^{\#},Q_n)&=&-(P_n-P_0)L_1(Q_n^{\#},Q_n)+P_n L_1(Q_n^{\#},Q_n)\\
&=&-(P_n-P_0)L_1(Q_n^{\#},Q_n)+O_P(n^{-1/2-\alpha(d)}),\end{eqnarray*}
by Theorem \ref{thnpbootmle}. The first term $(P_n-P_0)L_1(Q_n^{\#},Q_n)=O_P(n^{-1/2-\alpha(d)})$ as well, as shown earlier.
Thus, we have shown
\[P_0 L_1(Q_{n,\tilde{\epsilon}_n^{\#}}^{\#})-P_0L_1(Q_0)=O_P(n^{-1/2-\alpha(d)}).\]
Thus, we have shown $d_{01}(Q_{n,\tilde{\epsilon}_n^{\#}}^{\#},Q_0)=O_P(n^{-1/2-\alpha(d)})$ and $\epsilon_n^{\#}-\tilde{\epsilon}_n^{\#}=O_P(n^{-1/2})$.
By using that $d_{01}(Q,Q_0)$ behaves as a  square of an $L^2(P_0)$-norm, it follows trivially that this implies $d_{01}(Q_{n,\epsilon_n^{\#}}^{\#},Q_0)=O_P(n^{-1/2-\alpha(d)})$.
